# Supplementary material for: One Shot 3D Photography
Source: arXiv:2008.12298 source file (2020-09-01)
Supplement: Supplementary file 1 [file supplementary.tex]

Below, we provide additional metrics for the depth evaluation, as well as a detailed description of the Tiefenrausch network.

\begin{table*}[!hb]
\centering
\caption{Depth evaluation.}
\label{tab:depth_eval}
\begin{adjustbox}{max width=\textwidth}
\definecolor{altcolor}{gray}{0.9}
\definecolor{ourcolor}{rgb}{0.8, 0.9, 0.8}
\begin{tabular}{lll|S[table-format=1.3]S[table-format=1.3]S[table-format=1.3]S[table-format=1.3]S[table-format=1.3]S[table-format=1.3]S[table-format=1.3]|S[table-format=1.3]S[table-format=1.3]S[table-format=1.3]S[table-format=1.3]S[table-format=1.3]S[table-format=1.3]S[table-format=1.3]}\toprule
&&& \multicolumn{7}{c|}{Quality (MegaDepth test split)} & \multicolumn{7}{c}{Quality (ReDWeb)}\\
Method & Training data & Resolution &
{$\delta\!<\!1.25\!\uparrow$} & {$\delta\!<\!1.25^2\!\uparrow$} & {$\delta\!<\!1.25^3\!\uparrow$} &
{Abs rel$\downarrow$} & {Sq rel$\downarrow$} & {siRMSE$\downarrow$} & {RMSE$\downarrow$} &
{$\delta\!<\!1.25\!\uparrow$} & {$\delta\!<\!1.25^2\!\uparrow$} & {$\delta\!<\!1.25^3\!\uparrow$} &
{Abs rel$\downarrow$} & {Sq rel$\downarrow$} & {siRMSE$\downarrow$} & {RMSE$\downarrow$}\\
\midrule
Midas (v1) & \small RW, MD, MV & 384 & 0.955 & 0.987 & 0.994 & 0.068 & 0.007 & 0.094 & 0.027 & 0.668 & 0.801 & 0.849 & 0.740 & 0.126 & 0.840 & 0.067\\
Midas (v2) & \small RW, DL, MV, MD, WSVD & 384 & 0.965 & 0.990 & 0.995 & 0.058 & 0.008 & 0.085 & 0.022 & 0.662 & 0.793 & 0.843 & 1.342 & 0.225 & 0.827 & 0.071\\
Monodepth2 & \small K & $1024\!\times\!320$ & 0.845 & 0.956 & 0.983 & 0.145 & 0.019 & 0.165 & 0.049 & 0.350 & 0.562 & 0.682 & 4.368 & 1.067 & 1.181 & 0.176\\
SharpNet & \small PBRS $\rightarrow$ NYUv2 & 640 & 0.839 & 0.956 & 0.983 & 0.146 & 0.017 & 0.167 & 0.051 & 0.308 & 0.529 & 0.663 & 6.616 & 1.892 & 1.221 & 0.196\\
MegaDepth & \small DIW $\rightarrow$ MD & 384 & 0.929 & 0.982 & 0.992 & 0.086 & 0.010 & 0.115 & 0.033 & 0.434 & 0.635 & 0.736 & 2.270 & 0.466 & 1.137 & 0.137\\
Ken Burns & \small MD, NYUv2, KB & 1024 & 0.948 & 0.985 & 0.993 & 0.070 & 0.008 & 0.107 & 0.026 & 0.438 & 0.634 & 0.734 & 2.968 & 0.632 & 1.067 & 0.140\\
PyD-Net & \small CS $\rightarrow$ K & 512 &
0.836 & 0.955 & 0.982 & 0.148 & 0.021 & 0.168 & 0.052 &
0.310 & 0.525 & 0.656 & 5.218 & 1.411 & 1.205 & 0.198\\
\midrule
%Tiefenrausch \small{(ours)} & \small MD & 384 & 0.934 & 0.980 & 0.991 & 0.082 & 0.009 & 0.141 & 0.032 & 0.358 & 0.575 & 0.694 & 1.580 & 0.371 & 1.223 & 0.162\\
Tiefenrausch \small{(ours)} & \small MD & 384 & 
%0.934 & 0.980 & 0.991 & 0.082 & 0.009 & 0.141 & 0.032 & 
 0.941 & 0.983 & 0.993 & 0.079 & 0.009 & 0.109 & 0.031 &
%0.358 & 0.575 & 0.694 & 1.580 & 0.371 & 1.223 & 0.162\\
 0.382 & 0.597 & 0.714 & 1.950 & 0.374 & 1.041 & 0.156\\
\bottomrule
\end{tabular}
\end{adjustbox}
\end{table*}

\begin{table*}[h]
\centering
\caption{Tiefenrausch model stage descriptions. As the network has multiple paths, the stages are labeled (e.g., 0A) and the inputs to the stages are indicated as Input Stage(s). TRB $K \times K$ is the efficient block structure with a kernel size of $K$. Repeat is the number of times the operator is repeated in that stage. In the case where repeat $>$ 1 and stride $>$ 1, only the initial block in the stage has stride $>$ 1. }
\label{table:tr_model}
\begin{adjustbox}{max width=\textwidth}

\begin{tabular}{cccccccc}
\toprule
Stage       & Input                 & Operator                    & Exp factor & Out Channels & Stride & Repeat & Input Stage(s)\\ 
\midrule
0A            & $3\times384\times288$  & Conv2d $3\times3$, BN, ReLU & -        & 48           & 1      & 1 & Input  \\
0B            & $48\times384\times288$ & TRB $3\times3$              & -        & 32           & 1      & 3 & 0A     \\
0C            & $32\times384\times288$ & Conv2d $3\times3$, BN, ReLU & -        & 1            & 1      & 1 & 0B, 1C \\

1A            & $48\times384\times288$ & TRB $3\times3$              & -        & 40           & 2      & 3 & 0B     \\
1B            & $40\times192\times144$ & TRB $3\times3$              & -        & 8            & 1      & 3 & 1A     \\
1C            & $8\times192\times144$  & TRB $3\times3$              & -        & 32           & 1      & 3 & 1B, 2C \\

2A            & $8\times192\times144$  & TRB $3\times3$              & 4        & 56           & 2      & 3 & 1B     \\
2B            & $56\times96\times72$   & TRB $3\times3$              & 4        & 56           & 1      & 3 & 2A     \\
2C            & $56\times96\times72$   & TRB $3\times3$              & 4        & 8            & 1      & 3 & 2B, 3C \\

3A            & $56\times96\times72$   & TRB $3\times3$              & 5        & 80           & 2      & 3 & 2B     \\
3B            & $80\times48\times36$   & TRB $3\times3$              & 5        & 96           & 1      & 3 & 3A     \\
3C            & $96\times48\times36$   & TRB $3\times3$              & 5        & 56           & 1      & 3 & 3B, 4C \\

4A            & $96\times48\times36$   & TRB $3\times3$              & 9        & 64           & 2      & 3 & 3B     \\
4B            & $64\times24\times18$   & TRB $3\times3$              & 9        & 96           & 1      & 3 & 4A     \\
4C            & $96\times24\times18$   & TRB $3\times3$              & 9        & 96           & 1      & 3 & 4B, 5C \\

5A            & $96\times24\times18$   & TRB $3\times3$              & 9        & 96           & 2      & 3 & 4B     \\
5B            & $96\times12\times9$   & TRB $3\times3$               & 9        & 96           & 1      & 3 & 5A     \\
5C            & $96\times12\times9$   & TRB $3\times3$               & 9        & 96           & 1      & 3 & 5B     \\

\bottomrule
\end{tabular}
\end{adjustbox}
\end{table*}
